# Supplementary material for: Updating CLIP to Prefer Descriptions Over Captions
Source: arXiv:2406.09458 source file (2024-10-03)
Supplement: Supplementary file 1 [file ig-appendix-examples.tex]

\begin{figure*}
    \centering
    \begin{minipage}{0.19\linewidth}
    \resizebox{!}{\textwidth}{
    \includegraphics{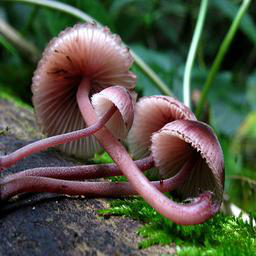}
    }
    \end{minipage}
    \begin{minipage}{0.78\textwidth}
    \resizebox{\textwidth}{!}{
      \centering
      \setlength{\tabcolsep}{4pt}
        \begin{tabular}{lccl}
        \toprule
        \textbf{Example} & \textbf{Mediation} & \textbf{Score} & \textbf{Attribution} \\
        \midrule
        \multirow{2}{*}{Description} & \xmark & +12.0 & \colorbox{green!5}{\strut a}\colorbox{green!1}{\strut cluster}\colorbox{green!0}{\strut of}\colorbox{green!21}{\strut pur}\colorbox{green!5}{\strut p}\colorbox{green!1}{\strut lish}\colorbox{green!6}{\strut -}\colorbox{green!8}{\strut red}\colorbox{green!100}{\strut mushrooms}\colorbox{magenta!0}{\strut on}\colorbox{magenta!2}{\strut their}\colorbox{magenta!0}{\strut sides}\colorbox{magenta!0}{\strut showing}\colorbox{magenta!3}{\strut the}\colorbox{magenta!0}{\strut under}\colorbox{magenta!3}{\strut side}\colorbox{green!0}{\strut of}\colorbox{magenta!1}{\strut their}\colorbox{magenta!5}{\strut caps}\colorbox{magenta!2}{\strut .} \\
        & \cmark & +5.77 & \colorbox{green!12}{\strut a}\colorbox{green!20}{\strut cluster}\colorbox{green!9}{\strut of}\colorbox{green!41}{\strut pur}\colorbox{green!17}{\strut p}\colorbox{green!19}{\strut lish}\colorbox{green!8}{\strut -}\colorbox{green!11}{\strut red}\colorbox{green!100}{\strut mushrooms}\colorbox{green!1}{\strut on}\colorbox{magenta!5}{\strut their}\colorbox{green!9}{\strut sides}\colorbox{magenta!0}{\strut showing}\colorbox{magenta!9}{\strut the}\colorbox{magenta!5}{\strut under}\colorbox{magenta!9}{\strut side}\colorbox{green!1}{\strut of}\colorbox{magenta!6}{\strut their}\colorbox{magenta!14}{\strut caps}\colorbox{magenta!7}{\strut .} \\
        \midrule
        \multirow{3}{*}{Caption} & \xmark & -2.95 & \colorbox{magenta!55}{\strut young}\colorbox{green!100}{\strut fruit}\colorbox{green!14}{\strut bodies}\colorbox{magenta!12}{\strut are}\colorbox{magenta!27}{\strut pru}\colorbox{green!1}{\strut ino}\colorbox{magenta!8}{\strut seas}\colorbox{magenta!31}{\strut if}\colorbox{green!14}{\strut covered}\colorbox{magenta!4}{\strut with}\colorbox{magenta!10}{\strut a}\colorbox{magenta!5}{\strut fine}\colorbox{magenta!32}{\strut white}\colorbox{magenta!20}{\strut powder}\colorbox{magenta!14}{\strut .} \\
        & \cmark & -2.99 &  \colorbox{magenta!100}{\strut young}\colorbox{green!87}{\strut fruit}\colorbox{green!18}{\strut bodies}\colorbox{magenta!18}{\strut are}\colorbox{magenta!50}{\strut pru}\colorbox{green!0}{\strut ino}\colorbox{magenta!2}{\strut seas}\colorbox{magenta!45}{\strut if}\colorbox{green!22}{\strut covered}\colorbox{green!2}{\strut with}\colorbox{magenta!11}{\strut a}\colorbox{magenta!1}{\strut fine}\colorbox{magenta!1}{\strut white}\colorbox{magenta!26}{\strut powder}\colorbox{magenta!25}{\strut .} \\
        \bottomrule
        \end{tabular}
    }
    \end{minipage}
    \begin{minipage}{0.19\linewidth}
    \resizebox{!}{\textwidth}{
    \includegraphics{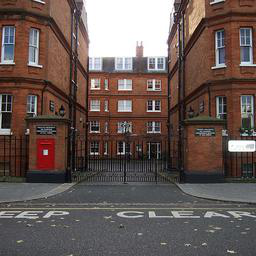}
    }
    \end{minipage}
    \begin{minipage}{0.78\textwidth}
    \resizebox{\textwidth}{!}{
      \centering
      \setlength{\tabcolsep}{4pt}
        \begin{tabular}{lccl}
        \toprule
        \textbf{Example} & \textbf{Mediation} & \textbf{Score} & \textbf{Attribution} \\
        \midrule
        \multirow{2}{*}{Description} & \xmark & +1.35 & \colorbox{green!14}{\strut a}\colorbox{magenta!88}{\strut block}\colorbox{green!53}{\strut of}\colorbox{green!100}{\strut flats}\colorbox{magenta!17}{\strut behind}\colorbox{magenta!36}{\strut a}\colorbox{magenta!32}{\strut set}\colorbox{magenta!6}{\strut of}\colorbox{magenta!8}{\strut high}\colorbox{green!21}{\strut security}\colorbox{green!77}{\strut gates} \\
        & \cmark & -1.38 & \colorbox{green!6}{\strut a}\colorbox{magenta!100}{\strut block}\colorbox{green!47}{\strut of}\colorbox{green!74}{\strut flats}\colorbox{magenta!9}{\strut behind}\colorbox{magenta!13}{\strut a}\colorbox{magenta!21}{\strut set}\colorbox{magenta!1}{\strut of}\colorbox{magenta!20}{\strut high}\colorbox{magenta!42}{\strut security}\colorbox{green!10}{\strut gates} \\
        \midrule
        \multirow{3}{*}{Caption} & \xmark & -7.85 & \colorbox{magenta!87}{\strut the}\colorbox{magenta!64}{\strut exclusive}\colorbox{magenta!95}{\strut block}\colorbox{green!11}{\strut of}\colorbox{green!0}{\strut flats}\colorbox{magenta!100}{\strut in}\colorbox{magenta!19}{\strut chelsea}\colorbox{magenta!53}{\strut ,}\colorbox{green!28}{\strut london}\colorbox{magenta!54}{\strut that}\colorbox{magenta!44}{\strut were}\colorbox{magenta!25}{\strut used}\colorbox{magenta!11}{\strut as}\colorbox{magenta!31}{\strut the}\colorbox{magenta!3}{\strut exterior}\colorbox{magenta!7}{\strut of}\colorbox{magenta!56}{\strut mark}\colorbox{magenta!59}{\strut 's}\colorbox{green!64}{\strut flat} \\
        & \cmark & -9.15 & \colorbox{magenta!75}{\strut the}\colorbox{magenta!59}{\strut exclusive}\colorbox{magenta!100}{\strut block}\colorbox{green!7}{\strut of}\colorbox{magenta!27}{\strut flats}\colorbox{magenta!68}{\strut in}\colorbox{magenta!48}{\strut chelsea}\colorbox{magenta!47}{\strut ,}\colorbox{magenta!35}{\strut london}\colorbox{magenta!41}{\strut that}\colorbox{magenta!38}{\strut were}\colorbox{magenta!30}{\strut used}\colorbox{magenta!10}{\strut as}\colorbox{magenta!27}{\strut the}\colorbox{magenta!18}{\strut exterior}\colorbox{magenta!9}{\strut of}\colorbox{magenta!47}{\strut mark}\colorbox{magenta!52}{\strut 's}\colorbox{green!48}{\strut flat} \\
        \bottomrule
        \end{tabular}
    }
    \end{minipage}
    \caption{Integrated gradient attributions for sample images and their corresponding description and caption from the Concadia dataset. A positive token attribution means that the token contributed positively to the outputted \clipscore\ (green), and negative token attribution means that it contributed negatively (magenta). The overall score is the sum of the token attributions within the sentence.}
    \label{fig:ig-appendix-examples}
\end{figure*}
